# Supplementary material for: Strong Interactions of Single Atoms and Photons near a Dielectric Boundary
Source: arXiv:1011.0740 ancillary file (2010-11-02)
Supplement: Supplementary file 1 [file Supplemental.pdf]

# Supplementary Information - Strong Interactions of Single Atoms and Photons near a Dielectric Boundary

D. J. Alton,[1] N. P. Stern,[1] Takao Aoki,[2] H. Lee,[3] E. Ostby,[3] K. J. Vahala,[3] and H. J. Kimble[1]

[1]*Norman Bridge Laboratory of Physics MC 12-33, California Institute of Technology, Pasadena, California 91125, USA*

[2]*Department of Physics, Kyoto University, Kyoto, Japan*

[3]*T. J. Watson Laboratory of Applied Physics MC 128-95, California Institute of Technology, Pasadena, California 91125, USA*

Supporting documentation of the experimental methods and theoretical modeling is provided for Ref. 1.

## I. THEORETICAL DESCRIPTION OF MICROTOROID CAVITY QED

Here we outline a cQED model for an atom coupled to a cylindrically symmetric resonator as originally presented in the supplementary material of Refs. 2 and 3 and shown schematically in Fig. S1. A microtoroidal cavity supports two degenerate counter-propagating whispering gallery modes at resonance frequency $\omega_c$ with annihilation operators $a$ and $b$, which are coupled via scattering at a rate $h$ [4]. Each travelling-wave mode has an intrinsic loss rate, $\kappa_i$, due to absorption, scattering, and radiation. A tapered fiber carries input fields $\{a_{\rm in}, b_{\rm in}\}$ at frequency $\omega_p$ which couple to the cavity modes with an extrinsic coupling rate $\kappa_{\rm ex}$. The output fields of the fiber taper can be written in terms of the input fields as $\{a_{\rm out}, b_{\rm out}\} = -\{a_{\rm in}, b_{\rm in}\} + \sqrt{2\kappa_{\rm ex}}\{a, b\}$ [2, 3]. For single-sided excitation, $\langle b_{\rm in}\rangle = 0$ and $a_{\rm in}$ drives the $a$ mode with strength $\varepsilon_p = i\sqrt{2\kappa_{\rm ex}}\langle a_{\rm in}\rangle$. The transmitted and reflected photon fluxes, $P_T = \langle a^\dagger_{\rm out} a_{\rm out}\rangle$ and $P_R = \langle b^\dagger_{\rm out} b_{\rm out}\rangle$, are calculated from the input flux $P_{\rm in} = \langle a^\dagger_{\rm in} a_{\rm in}\rangle$, with the transmission and reflection coefficients defined as $T = P_T/P_{\rm in}$ and $R = P_R/P_{\rm in}$, respectively.

We consider a two-level atom with transition frequency $\omega_a$ at location $\vec{r}(\rho, \phi, z)$ (in standard cylindrical coordinates) coupled to the travelling wave modes $\{a, b\}$ with single-photon coupling rate $g_{\rm tw}(\vec{r}) = g_{\rm tw}^{\max} f(\rho, z) e^{\pm i\theta}$, where $f(\rho, z)$ is a function determined by the cavity mode, $\theta = k\rho\phi$, and $k$ is the wavevector of the circulating mode. The atomic frequency $\omega_a$ may in general be shifted from the free-space value $\omega_a^{(0)}$ by frequency $\delta_a$ from the vacuum frequency due to interactions with the dielectric resonator. An approximate form for the function $f(\rho, z)$ for the lowest order toroid mode in the evanescent region can be written as $f(\rho, z) \sim e^{-d/\lambda} e^{-(\psi/\psi_0)^2}$ where $d = d(\rho, z)$ is the closest distance to the toroid surface, $\psi(\rho, z)$ is the angle around the toroid $\rho - z$ cross-section ($\psi = 0$ at $z = 0$), $\psi_0$ is a characteristic angle, and $\lambda_0 \equiv \lambda_0/2\pi$ where $\lambda_0$ is the free-space wavelength.

The Hamiltonian in a frame rotating at $\omega_p$ is given by [2–4]:

$$\begin{aligned} H/\hbar =& \Delta_{\rm ap}\sigma^+\sigma^- + \Delta_{\rm cp}\left(a^\dagger a + b^\dagger b\right) \\ &+ h\left(a^\dagger b + b^\dagger a\right) + \varepsilon_p^* a + \varepsilon_p a^\dagger \\ &+ \left(g_{\rm tw}^* a^\dagger \sigma^- + g_{\rm tw}\sigma^+ a\right) + \left(g_{\rm tw} b^\dagger \sigma^- + g_{\rm tw}^* \sigma^+ b\right) \end{aligned} \quad (1)$$

where $\sigma^\pm$ are the atomic raising and lowering operators, $\Delta_{\rm ap} = \omega_a - \omega_p$ and $\Delta_{\rm cp} = \omega_c - \omega_p$. Dissipation is treated using the master equation for the density operator of the system $\rho$:

$$\begin{aligned} \dot{\rho} =& -\frac{i}{\hbar}[H, \rho] + \kappa\left(2a\rho a^\dagger - a^\dagger a\rho - \rho a^\dagger a\right) \\ &+ \kappa\left(2b\rho b^\dagger - b^\dagger b\rho - \rho b^\dagger b\right) \\ &+ \gamma\left(2\sigma^-\rho\sigma^+ - \sigma^+\sigma^-\rho - \rho\sigma^+\sigma^-\right) \end{aligned} \quad (2)$$

Here, $\kappa = \kappa_i + \kappa_{\rm ex}$ is the total field decay rate of each cavity mode, and $2\gamma(\vec{r})$ is the atomic spontaneous emission rate, which is orientation dependent near a dielectric surface (Sec. III B 2). The Hamiltonian (Eq. 1) can be rewritten in a standing wave basis using normal modes $A = (a + b)/\sqrt{2}$ and $B = (a - b)/\sqrt{2}$,

$$\begin{aligned} H/\hbar =& \Delta_{\rm ap}\sigma^+\sigma^- + (\Delta_{\rm cp} + h)A^\dagger A + (\Delta_{\rm cp} - h)B^\dagger B \\ &+ \left(\varepsilon_p^* A + \varepsilon_p A^\dagger\right)/\sqrt{2} + \left(\varepsilon_p^* B + \varepsilon_p B^\dagger\right)/\sqrt{2} \\ &+ g_A\left(A^\dagger\sigma^- + \sigma^+ A\right) - ig_B\left(B^\dagger\sigma^- - \sigma^+ B\right) \end{aligned} \quad (3)$$

where $g_A(\vec{r}) = g_{\max} f(\rho, z)\cos\theta$, $g_B(\vec{r}) = g_{\max} f(\rho, z)\sin\theta$, and $g_{\max} = \sqrt{2} g_{\rm tw}^{\max}$. Depending on the azimuthal coordinate $\theta$, coupling may occur predominantly, or even exclusively, to one of the two normal modes. For such $\theta$, the system can be interpreted as an atom coupled to one normal mode in a traditional Jaynes-Cummings model with dressed-state splitting given by the single-photon Rabi frequency $\Omega_{(1)} = 2g \equiv 2g_{\max} f(\rho, z)$, along with a second complementary cavity mode not coupled to the atom. For a fixed phase of $h$ set by the scattering in the toroid, this decomposition is not possible for arbitrary atomic coordinate $\theta$; for non-zero $h$ the atom in general couples to both normal modes as $\theta$ is varied [2].

The master equation can be numerically solved using a truncated number state basis for the cavity modes. Alternatively, for sufficiently weak probe field, Eq. (2) can be linearized to find equations of motion for the field amplitudes. Note that while the detunings $\Delta_{\rm cp}$ and $\Delta_{\rm ap}$ in these theoretical expressions are referenced to the probe frequency, those used in the main text are referenced

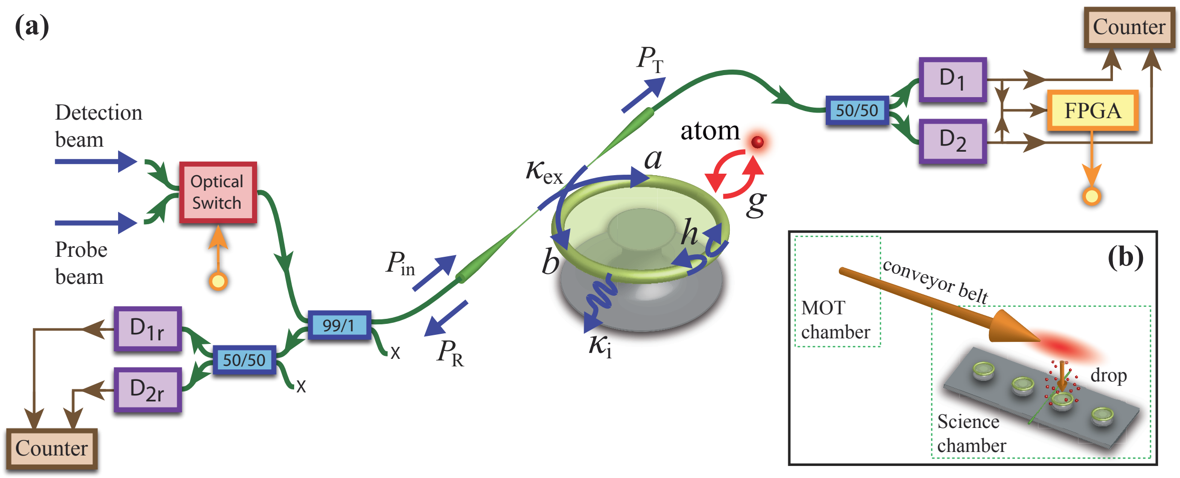


FIG. S1. Schematic of microtoroidal cQED system. (a) A microtoroidal resonator supports counter-propagating travelling wave modes $\{a, b\}$ coupled at a rate $h$. The circulating fields decay at a rate $\kappa = \kappa_i + \kappa_{ex}$ where $\kappa_i$ is the resonator intrinsic loss rate and $\kappa_{ex} = \sqrt{\kappa_i^2 + h^2}$ is the coupling rate between the cavity and a tapered fiber at critical coupling. An optical switch controlled by an FPGA selects the probe beam conditioned upon detection of an atom coupled to the cavity modes (Section IIA). The all-in-fiber switch and beam splitter network delivers a power $P_{in}$ to the microtoroid. Transmitted power $P_T$ and reflected power $P_R$ are detected by four single photon counting modules (SPCMs) and digitally recorded by a counter card. (b) A cloud of cesium atoms from a separate 'MOT chamber' is transferred via a differential pumping tube by an optical conveyor belt into the 'Science chamber' and released 800 $\mu$m above a microtoroid.

to the free-space frequency $\omega_a^{(0)}$ of the $6S_{1/2}, F = 4 \to 6P_{3/2}, F' = 5$ transition of Cs.

## II. EXPERIMENTAL DETAILS

The experimental setup is similar to that in Ref. 5 and is illustrated in Fig. S1. Briefly, Cesium atoms are magneto-optically cooled and trapped in a 'MOT chamber', then loaded into an optical conveyor belt [6], and transported over 20 cm into a 'Science chamber' (at $< 10^{-9}$ Torr) through a differential pumping tube to limit cesium contamination on the microtoroids [5]. This cloud of $\sim 10^7$ atoms at temperature $T \approx 100$ $\mu$K is dropped 800 $\mu$m directly above a microtoroid. Access to the input and output light fields of the microtoroid is provided by a tapered optical fiber. The taper and toroid chip are mounted on piezoelectric-driven stages inside the 'Science' chamber that enable stable tuning of $\kappa_{ex}$ to the critical coupling condition $\kappa_{ex} = \sqrt{\kappa_i^2 + h^2}$ for which the transmitted output flux $P_T$ nearly vanishes for $\Delta_{cp} = 0$. In practice, a darkness of $T = P_T/P_{in} \approx 0.01$ at critical coupling is maintained.

Detection and probe beams pass through fast ($\sim 10$ ns response) in-fiber Mach-Zehnder optical switches before entering a beam splitter network which reduces the power to $P_{in}$ (Fig. S1 (a)). The transmitted beam $P_T$ passes through a 50/50 beam-splitter to two single-photon counting-modules (SPCMs), $\{D_1, D_2\}$, while the reflected beam $P_R$ travels back through the beam splitter network to another two SPCMs, $\{D_{1r}, D_{2r}\}$. The photon count time series $C_i(t)$ from detector $D_i$ is recorded on a photon counting card with 2-ns resolution. In each experimental cycle, a detection beam with $\omega_p = \omega_c$ is used for real-time atom detection while the atom cloud is falling (see Sec. II A). The atom cloud takes $\sim 50$ ms to pass the toroid, during which $1 - 10$ single atom events each typically lasting 2-4 $\mu$s are observed. Upon a trigger event determined by a 40-MHz field-programmable gate array (FPGA), the fiber input is switched from the detection to the probe beam, which can have different power and/or frequency detuning. The entire sequence from MOT loading through atom dropping takes $\sim 500$ ms. During the $\sim 450$ ms when atoms are not falling, a third beam with frequency continuously scanned over a range of $\sim 1$ GHz around $\omega_a^{(0)}$ is used to measure $\omega_c$. The empty cavity transmission measured with this scanning beam is also used to optimize the cavity-fiber coupling, $\kappa_{ex}$.

A silicon chip with 10 silica microtoroids is fabricated using standard methods [7] and mounted on a thermo-electric heat pump for coarse temperature control. An optical heating servo with $\sim 10$-Hz bandwidth stabilizes the resonance frequency $\omega_c$ for the mode of interest to within $\sim 1$ MHz of $\omega_a^{(0)}$. The microtoroid used in the experiment has a principal diameter of $D_p \approx 24$ $\mu$m, minor diameter of $D_m \approx 3$ $\mu$m, and a quality factor $Q \sim 10^7$. A finite element model of the fundamental TE mode for this geometry gives a mode volume of $\sim 100$ $\mu m^3$, corresponding to maximum atom-cavity coupling for linear polarized light of $g_{max}/2\pi \approx 150$ MHz at the toroid surface. The parameters for the $\Delta_{ca} = 0$ and $\Delta_{ca}/2\pi = 60$ MHz measurements are $(\kappa_i, h, \kappa_{ex})/2\pi = (8, 10, 12.8)$ MHz, and for the $\Delta_{ca}/2\pi = \pm 40$ MHz measurements are $(\kappa_i, h, \kappa_{ex})/2\pi = (13.5, 11, 17.4)$ MHz. For the results of Ref. 1, the typical intracavity photon number is $\bar{n} \lesssim 0.1$ in the absence of an atom and the effective mean atom-cavity coupling is $\bar{g}/2\pi \approx 40$ MHz. For $\kappa/2\pi \sim 20$ MHz, the critical photon number $n_0 \approx \gamma_0^2/2\bar{g}^2 \sim 10^{-3}$ and crit-

ical atom number $N_0 \approx 2\gamma_0\kappa/\bar{g}^2 \sim 10^{-2}$ are both less than unity. With $\bar{g} > (\kappa, \gamma_0)$, the system is in the single photon, strong coupling regime.

### A. Real-time detection of atom transits

The temporal and spectral experiments described in Ref. 1 are realized by switching the driving laser conditioned on a single atom being sufficiently well-coupled to the cavity to measure an appreciable response. Real-time detection and triggering of atomic transits is achieved in less than a microsecond for atom transits which typically last a few microseconds so that the optical triggering and switching occur while the atom remains coupled to the resonator. Single-atom detection is performed at critical coupling with $P_{\rm T} \leq 0.01 P_{\rm in}$. When an atom is coupled to the cavity, the cQED eigenstructure splits and $P_{\rm T}$ increases. The cavity response for $\Delta_{\rm ca} = 0$ is shown for representative values of azimuthal location $\theta$ in Fig. S2 (a)-(b), illustrating the increase in $T$ for $g \neq 0$ and the sensitivity to $\theta$. The spectra vary smoothly with $\theta$, with $\theta = \pi/2$ the mirror image about $\Delta_{\rm pa} = 0$ of $\theta = 0$. During the 50-ms interval after Cs atoms are released, $P_{\rm T}$ is monitored by SPCMs $D_1$ and $D_2$ and analyzed in real-time by a 40-MHz FPGA. The FPGA outputs a trigger pulse when it counts a threshold $C_{\rm th}$ single-photon pulses in a running time window of length $\Delta t_{\rm th}$. The trigger gates the photon counting card as well as controls the optical switch network. Signal logic, electrical and optical travel times, and optical switch times introduce a latency of approximately 100 ns between trigger and modulation of probe beam parameters at the toroid.

Figures S2 (c) and (d) show the transmitted flux $\sum (C_1(t) + C_2(t))$ summed over 1501 triggers using $C_{\rm th} = 4$ and $\Delta t_{\rm th} = 750$ ns. For these measurements, instead of switching the input beam upon a trigger event, the FPGA trigger times are digitally recorded along with the photon counts. In part (c), the time series $C_1(t) + C_2(t)$ for each trajectory is aligned such that the trigger occurs at $t = 0$. The sharp peak just before $t = 0$ has a width of $\sim 50$ ns, corresponding to the last (fourth) photon count that generated the trigger within the last 25-ns FPGA time step for every trigger. The previous three photon counts are distributed within the 750 ns window prior to the trigger. Note that 25 ns prior to the $\Delta t_{\rm th}$ window, $C_1 + C_2 = 0$ because if there were a count here, then the transit criteria would have been satisfied one 25-ns time step earlier. These classical detection biasing effects are not indicative of cQED dynamics of the microtoroidal system. In part (d), the time origin is determined for each trigger individually so that $t = 0$ corresponds to the weighted mean of photon arrival times for $\pm 10\ \mu$s around each trigger event. The distribution of the 1501 events shows that most of the triggers occur near the peak of the unconditional counts $C_1 + C_2$. For experiments, the trigger parameters $C_{\rm th}$ and $\Delta t_{\rm th}$ are chosen so that the false detection rate of atom triggers is below 1% and the trigger time is as early as possible relative to the peak trajectory transmission. For the experiments in Fig. 3 and 4 of the main text, we use the parameters $C_{\rm th} = 5$ and $\Delta t_{\rm th} = 750$ ns.

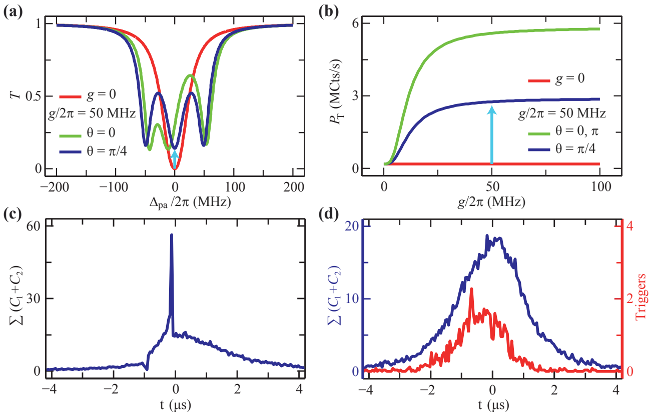


FIG. S2. Realtime detection of single atom transits. (a) Normalized transmission spectra $T(\Delta_{\rm pa}) = P_{\rm T}/P_{\rm in}$ as a function of probe detuning $\Delta_{\rm pa}$ for $g = 0$ and $g/2\pi = 50$ MHz ($\theta = 0$ and $\theta = \pi/4$) at critical coupling. The spectrum for $\theta = \pi/2$ is the mirror about the $\Delta_{\rm pa} = 0$ axis of the $\theta = 0$ case. (b) Transmitted photon flux as a function of $g$ for $\Delta_{\rm pa} = 0$. An atom trajectory with increasing $g$ (e.g., from $g = 0$ to $g/2\pi = 50$ MHz) results in increased $P_{\rm T}$ illustrated by the cyan arrow. (c) Experimental counts $C_1(t) + C_2(t)$ for 1501 transits from 596 atom drops with 4% false detection rate where the triggers are aligned at $t = 0$. (d) The same data aligned by redefining $t = 0$ to be the mean photon arrival time for each individual transit (blue). This alignment removes selection biasing seen in panel (c) and allows plotting of the distribution of trigger times relative to the transit center (red). Most triggers occur just prior to the peak transmission for the unconditional average over all atom transits. The data in (c) and (d) have been smoothed over a running window of 20 ns for clarity. In (b), (c) and (d) the maximum off-resonant transmitted photon flux (for $\Delta_{\rm cp} \gg \kappa_{\rm ex}$) is $P_{\rm T} \approx 1.8 \times 10^7$ counts/s $\sim 4$ pW.

## III. MODELING ENSEMBLES OF ATOMS DETECTED IN REAL TIME

The stochastic nature of the detection process used in Ref. 1 introduces an ensemble of cQED parameters included in any given measurement. We present two methods in this manuscript for understanding the resulting distributions. A simplified analytic approach gives a rough result by neglecting forces other than gravity on falling atoms. A Monte Carlo simulation treats atomic motion in a semiclassical model to investigate the effects of forces on the atoms, including radiation and surface forces.

### A. Analytic model for real-time detection distributions

Here we outline a simple analytic model of the stochastic distribution $p_{\rm fall}(g)$ of coupling parameters $g$ observed in a real-time detection experiment. We assume atoms fall vertically through a Gaussian cavity mode so that $g(\rho, z(t)) \sim g_{\rm c}(\rho) e^{-(z(t)/z_0)^2}$ with constant velocity so

that $z \propto t$ where $g_c(\rho) \sim g_{\max} e^{-(\rho - D_p)/\lambda_0}$ is the maximum coupling at closest approach. This simple approach neglects forces on the atom which significantly modify the atomic trajectories and the dynamics of real-time triggering (see Sec. III B).

Within the cQED model, the cavity transmission $T(\Delta_{\rm pa}, g(\vec{r}))$ is a known function of probe detuning and atom location $\vec{r}$. For this calculation, we assume that $\theta$ is restricted to values which maximize $T(\theta)$ at cavity resonance ($\theta = \pi/2$ for $\Delta_{\rm ca}/2\pi = +40$ MHz, for example). For simplicity, we also assume that the atoms are slowly moving so that the coupling at a trigger event is the only $g$ that contributes to a spectrum. The probability density function $p_{\rm fall}(g)$ can be estimated as the product of the probability of any atom having a particular $g$ and the probability of a trigger event occurring for an atom with coupling $g$, $p_{\rm fall}(g) \sim p_{\rm atom}(g) p_{\rm trigger}(g)$. An atom transit is triggered when the total detected photon counts exceeds a threshold number, $C_{\rm th}$, within a detection time window $\Delta t_{\rm th}$. The detection probability $p_{\rm trigger}(g)$ is estimated from a Poisson distribution of mean count $T(g) P_{\rm in} \Delta t_{\rm th}$. Given the Gaussian form of $g(t)$, $p_{\rm atom}(g)$ can be written as a product of the probability of $g$ in an atom transit with given $g_{\max}$ and the probability of a transit to have that $g_{\max}$, $p_{\max}(g_{\max})$, integrated over all $g_{\max}$,

$$p_{\rm atom}(g) = \int_g^{g_{\max}} p(g|g_{\rm c}) p_{\max}(g_{\rm c}) dg_{\rm c}. \qquad (4)$$

Note that the integral has limits from $g$ to $g_{\max}$ since $g_{\rm c}$ cannot be smaller than $g$. Analytic approximations for the form of $p_{\max}(g_{\rm c})$ and $p(g|g_{\rm c})$ can be found from the Gaussian approximation to the mode evanescent field so that Eq. 4 can be evaluated (see Fig. S3).

### B. Full Monte Carlo simulation

Analysis of experimental results which includes the details of atomic trajectories is implemented with a Monte Carlo simulation of atom transits near the toroid. For each desired set of experimental parameters, a set of atomic trajectories is generated which satisfies the stochastic detection criteria. This ensemble is used to extract the cavity output functions $T(t, \Delta_{\rm pa})$ and $R(t, \Delta_{\rm pa})$. For determining triggers with, $P_{\rm T} \sim |\langle a_{\rm out}\rangle|^2$ is calculated from a linearized approximation to Eq. 2. Numerical solution of the master equation verifies this method is accurate under the conditions of the experiment and with $\Delta_{\rm pa} \sim 0$. For spectral calculations, the flux $P_{\rm T} = \langle a^\dagger_{\rm out} a_{\rm out}\rangle$ is calculated from numerical solution of the master equation.

Since the spontaneous emission recoil velocity $\hbar k/m \sim 0.4$ cm/s is much less than the typical velocities of falling atoms $\sim 17$ cm/s at $z = 0$, we use a semiclassical approximation for atomic motion. The initial atomic velocity $\vec{v}_i$ is selected from the Maxwell-Boltzmann distribution of temperature $T = 100$ $\mu$K and the individual trajectories are propagated forward in time. Gravity, optical dipole

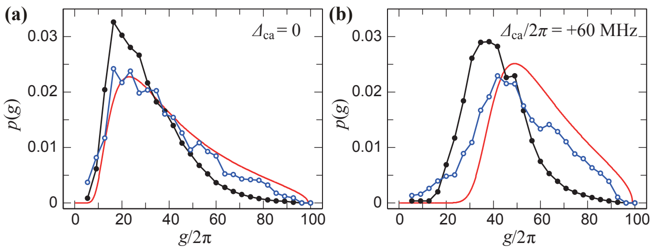


FIG. S3. Sample distributions $p(g)$ calculated for (a) $\Delta_{\rm ca}/2\pi = 0$ and (b) $\Delta_{\rm ca}/2\pi = +60$ MHz. The analytic model (red), the corresponding distribution from the Monte Carlo model with $U_{\rm d} = U_{\rm s} = 0$ (blue), and the distribution from the full Monte Carlo simulation with all potentials (black) are shown for comparison. The additional forces shift the distribution toward lower $g$, with large effect for $\Delta_{\rm ca} \neq 0$.

forces (Sec. III B 1), and Casimir-Polder surface interactions (Sec. III B 3) are included in the trajectory simulation. Selection logic simulating the FPGA criteria is applied to the photon counts from each trajectory, which are assumed to be Poissonian on the relevant timescales. The simulation is repeated to acquire enough triggered trajectories for a sufficient ensemble average for the final model output, which is typically at least 400 unique triggered trajectories. Spectral and temporal behaviors are calculated from the set of triggered trajectories generated for each detection criteria. The simulated output fluxes $P_{\rm T}(t)$ and $P_{\rm R}(t)$ are summed over the entire set of trajectories in the same time windows used for the experimental data to obtain the simulation results quoted in the text. A comparison of the distribution of $g$ between the simple analytic model of Sec. III A and the Monte Carlo simulation with and without forces appears in Fig. S3.

#### 1. *Dipole force*

The dipole force is calculated from the commutator $\vec{F} = \frac{d\vec{p}}{dt} = \frac{i}{\hbar}[H, \vec{p}]$ using the Hamiltonian Eq. 1. In order to make this operator expression tractable, operator products are calculated as products of linearized steady-state expectation values which is a reasonable approximation for weak driving power $P_{\rm in}$ [8, 9]. Momentum diffusion is implemented using a generalized expression for the atom-cavity diffusion tensor [10], again simplifying with linearized steady-state field expectation values. Although included in the trajectory model, diffusion is not a significant factor in falling atom trajectories at the power levels and atomic velocities in this experiment. For Fig. 1 of the main text, the effective potential $U_{\rm d}$ is calculated by integrating the dipole force along the path $\rho' = \infty \to \rho$, assuming all steady-state fields change adiabatically with atom location $\vec{r}$.

#### 2. *Spontaneous emission rate near a surface*

When a classical oscillating dipole is placed near a dielectric or metallic surface, its spontaneous emission rate is modified by the boundary. This behavior is in general

oscillatory with distance $d$ and dependent on the orientation, whether the dipole is parallel or perpendicular to the surface. The spontaneous emission rate features a marked increase within a wavelength of the surface due to available evanescent modes for decay. Calculations of $\gamma_{\|}(d)$ and $\gamma_{\perp}(d)$ for a planar surface used in our simulations and seen in Fig. 1(b) of the main text follow those of Ref. 11.

### 3. *Casimir-Polder interactions*

Casimir-Polder (CP) interactions are important components of atomic motion for neutral atoms within a few hundred nm of a surface [12]. For an atom located a small distance $d \ll \lambda$ from a dielectric surface, the potential takes the Lennard-Jones (LJ) form $U_{\rm s}^{\rm LJ} = -C_3/d^3$ where $C_3$ is a constant that depends on the atomic polarizability and dielectric permittivity of the surface [13, 14]. At larger distances, relativistic retardation [15] leads to a reduced potential $U_{\rm s}^{\rm ret} = -C_4/d^4$. Microtoroid cQED distance scales are set by the evanescent field scale length, $\lambda = 136$ nm (for the Cs $D2$ line). The relevant distances ($0 < d \lesssim 300$ nm) span both the LJ and retarded regimes, and consequently, the limiting power laws do not fully describe experimentally accessible CP interactions. Our model utilizes a full calculation of $U_{\rm s}$ with the Lifshitz equation [16, 17] valid over the entire range of $d$.

The CP potentials enter into our simulation in two distinct ways. First, the transition frequency $\omega_{\rm a}$ of the two-level atomic system shifts away from the vacuum frequency by $\delta_{\rm a} = (U_{\rm s}^{\rm ex}(\vec{r}) - U_{\rm s}^{\rm g}(\vec{r}))/\hbar$, where $U_{\rm s}^{\rm g}(\vec{r})$ and $U_{\rm s}^{\rm ex}(\vec{r})$ are the surface potentials for the ground and excited states, respectively. Second, a force $\vec{F}_{\rm s}(\vec{r}) = -\nabla U_{\rm s}(\vec{r})$ on the atom can be derived from these potentials.

We now briefly describe our calculation to find $U_{\rm s}^{\rm g}$ for a cesium atom near a $SiO_2$ glass surface. The frequency dependent polarizability of the Cs ground state $\alpha(\omega)$ and the complex dielectric function $\epsilon(\omega)$ of the silica surface are needed in the Lifshitz equation. $\epsilon(\omega)$ for $SiO_2$ is obtained from a fit of experimental data for the complex index of refraction [18] to a seven-oscillator Lorentz model. $\alpha(\omega)$ is calculated as a sum of Lorentz oscillators over valence 6S $\rightarrow$ $N$P transitions, with $N = 6 - 11$, whose oscillator strengths are tabulated in many sources [19]. A single high-frequency oscillator representing the Cs core polarizability is introduced with parameters such that the calculation matches the experimentally known ground state static polarizability $\alpha(0) = 5.942 \times 10^{-23}$ cm$^3$ [20] as well as the known ground state $C_3$ constant for a Cs atom near a metallic surface $C_3 = -\frac{\hbar}{4\pi d^3}\int_0^\infty \alpha(i\xi)d\xi = 4.4 \cdot h$ kHz $\mu$m$^3$ [21, 22]. For $U_{\rm s}^{\rm ex}$ we use the same core polarizability but use 6P $\rightarrow$ $N$S, $N$D valence states. Curvature of the silica surface is treated following the modified method of Ref. 24 with the toroid taken as a cylinder with radius of curvature $R = D_m/2$ using the calculated material properties $\epsilon(\omega)$ and $\alpha(\omega)$. Numerical evaluation of the excited state potential $U_{\rm s}^{\rm ex}$ is calculated in a similar manner as $U_{\rm s}^{\rm g}$, with an additional contribution accounting for real allowed photon exchange with the surface [23].

Figure S4 shows the atom-surface potential $U_{\rm s}^{\rm g}$ for the ground state of cesium near a $SiO_2$ surface. For the limiting cases, our calculation yields $C_3/h = 1178$ Hz $\mu$m$^3$ and $C_4/h = 158$ Hz $\mu$m$^4$ for a planar dielectric surface. Note that the transition region between LJ and retarded regimes dominates the relevant distance scales around 100 nm for our experiment, with $U_{\rm s}$ never fully reaching the CP power law behavior before the thermal limit takes over. For $d > D_m$, the curvature correction is no longer accurate [24], but in this regime, CP forces are already negligible to atomic motion. The excited state potential $U_{\rm s}^{\rm ex}$ has a similar form but is larger in magnitude.

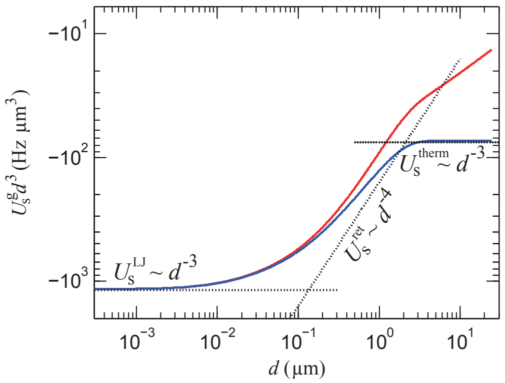


FIG. S4. Calculated atom-surface potential $U_{\rm s}^{\rm g}$ for a cesium atom at distance $d$ from a $SiO_2$ surface with radius of curvature $R = D_m/2 = 1.5$ $\mu$m (red) and $R \rightarrow \infty$ (blue). The limiting cases for $R \rightarrow \infty$ are shown as dotted lines. In the region where surface forces are important, the cylindrical correction provides an accurate expression for the CP potentials. For $d > R$, the cylindrical correction formula is no longer valid.


[1] see Alton, D. J., Stern, N. P., Aoki, T., Lee, H., Ostby, E., Vahala, K. J., and Kimble, H. J. Strong interactions of single atoms and photons near a dielectric boundary, (2010).

[2] Aoki, T., *et al.* Observation of strong coupling between one atom and a monolithic microresonator. *Nature* **442**, 671-674 (2006) and the associated supplementary material.

[3] Dayan, B., *et al.* A photon turnstile dynamically regulated by one atom. *Science* **319**, 1062-1065 (2008) and the associated supplementary material.

[4] Srinivasan, K. and Painter, O. Mode coupling and cavity-quantum-dot interactions in a fiber-coupled microdisk cavity. *Phys. Rev. A* **75**, 023814 (2007).

[5] Aoki, T., *et al.* Efficient routing of single photons by one atom and a microtoroidal cavity. *Phys. Rev. Lett.* **102**, 083601 (2009).

[6] Kuhr, S., Alt, W., Schrader, D., Müller, M., Gomer, V.,

and Meschede, D. Deterministic delivery of a single atom. *Science* **293**, 278-280 (2001).

[7] Armani, D. K., Kippenberg, T. J., Spillane, S. M., and Vahala, K. J. Ultra-high-Q toroid microcavity on a chip. *Nature* **421**, 925-928 (2003).

[8] Fischer, T., Maunz, P., Puppe, T., Pinkse, P.W.H., and Rempe, G. Collective light forces on atoms in a high-finesse cavity. *New J. Phys.*, **3**, 11 (2001).

[9] Doherty, A.C., Parkins, A. S., Tan, S. M., and Walls, D. F. Motion of a two-level atom in an optical cavity. *Phys. Rev. A*, **56**, 833 (1997).

[10] Murr, K., *et al.* Momentum diffusion for coupled atom-cavity oscillators. *Phys. Rev. A*, **74**, 043412 (2006).

[11] Lukosz, W. and Kunz, R. E. Light emission by magnetic and electric dipoles close to a plane interface. I. Total radiated power. *J. Opt. Soc. Am.*, **67**, 1607-1615 (1977).

[12] Sukenik, C. I., Boshier, M. G., Cho, D., Sandoghdar, V., and Hinds, E. A. Measurement of the Casimir-Polder force. *Phys. Rev. Lett.* **70**, 560 (1993).

[13] London, F. The general theory of molecular forces. *Trans. Faraday Soc.*, **33**, 8-26 (1937).

[14] Lennard-Jones, J. E. Processes of adsorption and diffusion on solid surfaces. *Trans. Faraday Soc.*, **28**, 334 (1932).

[15] Casimir, H. B. G. and Polder, D. The influence of retardation on the London-van der Waals forces. *Phys. Rev.*, **73**, 360-372 (1948).

[16] Lifshitz, E. M. The theory of molecular attractive forces between solids. *Sov. Phys. JETP*, **2**, 73-83 (1956).

[17] Dzyaloshinskii, I. E., Lifshitz, E. M., and Pitaevskii, L. P. General theory of van der Waals' forces. *Sov. Phys. Uspekhi*, **73**, 153-176 (1961).

[18] Philipp, H. R., "Silicon dioxide ($SiO_2$) (glass)," in *Handbook of Optical Constants of Solids*, E. D. Palik, ed. (Academic, Orlando, Fla., 1985), pp. 749-764.

[19] Norcross, D. W. Photoabsorption by cesium. *Phys. Rev. A*, **7**, 606 (1973).

[20] Amini, J. and Gould, H. High precision measurement of the static dipole polarizability. *Phys. Rev. Lett.*, **91**, 153001 (2001).

[21] Johnson, W. R., Dzuba, V. A., Safronova, U.I., and Safronova, M. S. Finite-field evaluation of the Lennard-Jones atom-wall interaction constant $C_3$ for alkali-metal atoms. *Phys. Rev. A*, **69**, 022508 (2004).

[22] Derevianko, A., Johnson, W.R., Safronova, M.S., and Babb, J.F. High-precision calculations of dispersion coefficients, static dipole polarizabilities, and atom-wall interaction constants for alkali-metal atoms. *Phys. Rev. Lett.*, **82**, 833 (1999).

[23] Fichet, M., Schuller, F., Bloch, D., and Ducloy, M. Van der Waals interaction between excited-state atoms and dispersive dielectric surface. *Phys. Rev. A*, **51**, 1553 (1995).

[24] Blagov, E. V., Klimchitskaya, G. L., and Mostepanenko, V. M. Van der Waals interaction between microparticle and uniaxial crystal with application to hydrogen atoms and multiwall carbon nanotubes. *Phys. Rev. B*, **71**, 235401 (2005).
